# Supplementary material for: Analyzing Commonsense Emergence in Few-shot Knowledge Models
Source: arXiv:2101.00297 source file (2021-09-10)
Supplement: Supplementary file 1 [file z-appendix.tex]

\documentclass[11pt,a4paper]{article}
\usepackage{akbc}
\usepackage{times}
\usepackage{latexsym}
\usepackage{amsmath}
\usepackage{amssymb}
\usepackage{enumitem}

% This is not strictly necessary, and may be commented out,
% but it will improve the layout of the manuscript,
% and will typically save some space.
\usepackage{microtype}
\usepackage{multirow}
\usepackage{graphicx}
\usepackage{float}
\usepackage{adjustbox}

\usepackage{physics}

\usepackage{xcolor}
\usepackage{soul}
\usepackage{booktabs}
\usepackage{relsize}

\usepackage[normalem]{ulem}
\useunder{\uline}{\ul}{}
\usepackage{tcolorbox}

%\aclfinalcopy % Uncomment this line for the final submission
 %  Enter the acl Paper ID here

%\setlength\titlebox{5cm}
% You can expand the titlebox if you need extra space
% to show all the authors. Please do not make the titlebox
% smaller than 5cm (the original size); we will check this
% in the camera-ready version and ask you to change it back.

\begin{document}

\include{sections/8-appendix}

\bibliography{emnlp2020}
\bibliographystyle{acl_natbib}

\end{document}
